# Supplementary material for: Shape Registration with Directional Data
Source: arXiv:1708.07791 ancillary file (2017-08-29)
Supplement: Supplementary file 1 [file supp.pdf]

# Shape Registration with Directional Data

Mairéad Grogan & Rozenn Dahyot
School of Computer Science and Statistics
Trinity College Dublin, Ireland

This document contains supplementary material for the paper 'Shape Registration with Directional Data'.

## I. More results for Section V

### A. 2D Rotation Registration (Section V-A)

- In Figure 1 we present a sample of the parametric curves used in our 2D shape registration experiments described in Section V-A of the paper. The curves are sampled at 50 different locations, with the normal vector at each point shown with a blue arrow.
- In Figure 2 we present some of the registration results computed using $\mathcal{C}^x$, $\mathcal{C}^u$ and $\mathcal{C}^{x,u}$ (column 1-3 respectively) when the curves differ by a rotation.
- In Figure 3 we present some of the registration results computed using $\mathcal{C}^x$, $\mathcal{C}^u$ and $\mathcal{C}^{x,u}$ (column 1-3 respectively) when the curves differ by a rotation and are missing data.

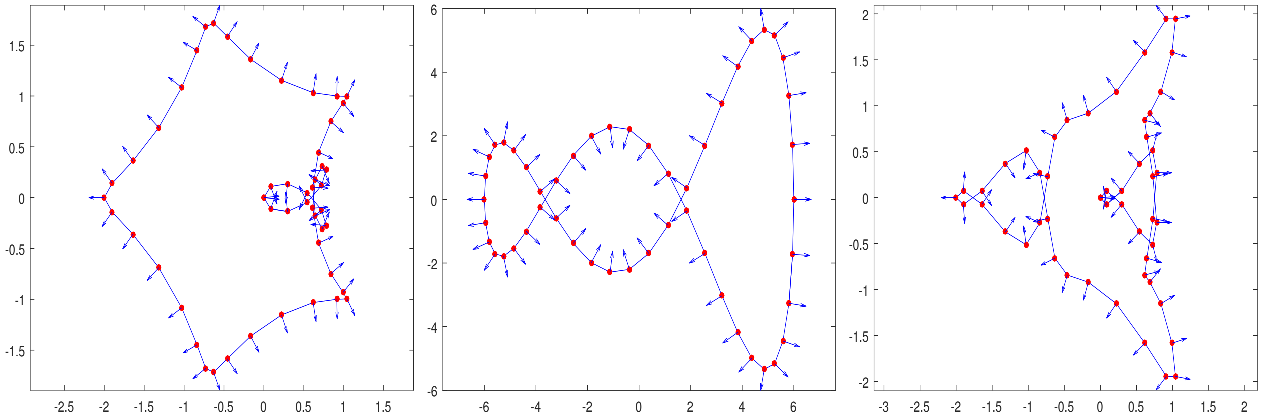

Fig. 1. Three different 2D parametric curves used in our experiments, sampled at 50 locations, along with their normal vectors.

### B. 2D Non-rigid Registration (Section V-B)

- Figure 4 details how we create the curves $S_1$ and $S_2$ for our experiments registering 2D curves differing by a non rigid deformation. Given a parametric curve $S_2$, we select 8 control points on the boundary of the curve. We move some of these control points, and compute the TPS transformation that maps the original set of control points onto the new set of control points. This transformation is applied to all points in the parametric curve $S_2$, deforming $S_2$ to create $S_1$. The number of control points that are moved determines the degree of the deformation applied to the curve.
- Figures 5, 6 and 7 show some of the registration results generated in our 2D non-rigid registration experiments. In Figure 5 we present results on curves differing by a non-rigid deformation. In Figure 6, we present results on curves differing by a non-rigid deformation and a rotation. In Figure 7 we present results on curves differing by a non-rigid deformation with missing data.

## II. More results for Section VI

### A. 3D Rotation Registration (Section VI-A)

- In Figure 8 we present the meshes used in our 3D registration experiments, the Bunny, Dragon, Buddha and Horse meshes (column 1). For each mesh we also show the distribution of their normal vectors on the 2D plane (column 2) and on the sphere (column 3).
- In Figure 9 we present the noisy point clouds which we register to noise free point clouds in our experiment described in Section VI-A.

### B. 3D Non-rigid Registration

- In Figure 10 we present a sample of the meshes used in our non-rigid experiment in 3D. Two meshes of the same animal (eg. cat, lion,horse) have the exact same number of vertices and have exact vertex correspondences.
- In Figure 11 we present some of the registration results generated when using $\mathcal{C}^{x}_{corr}$ and $\mathcal{C}^{x,u}_{corr}$ to register the point clouds. We found that the search space was too high for both $\mathcal{C}^{x}_{corr}$ and $\mathcal{C}^{x,u}_{corr}$, and the algorithms were stopped before the global minimum was found.
- In Figure 12 we present some of the registration results generated when using CPD, GLMD, $\mathcal{C}^{x}_{corr}$ and $\mathcal{C}^{x,u}_{corr}$ to register 3D shapes differing by a non rigid deformation only (columns 1 and 2) and a non-rigid deformation with a rotation (column 3). In this case, when using $\mathcal{C}^{x}_{corr}$ and $\mathcal{C}^{x,u}_{corr}$, vertex correspondences are estimated.

## III. More results for Section VII

In Figures 13 and 14 we present more results similar to those presented in Figure 7 of the paper. Again, the results generated using $\mathcal{C}^{x}$ are presented in (a) in both figures, and those generated using $\mathcal{C}^{x,u}$ are presented in (b), with $\mathcal{C}^{x,u}$ outperforming $\mathcal{C}^{x}$ in all cases.

## IV. Parameters Used

In this section we provide the parameters used for all methods tested in Sections V, VI and VII. When comparing with state of the art registration methods (Go ICP [1], CPD [2] and GLMD[3]) we use the parameters provided in the code supplied by the authors.

### A. 2D Rotation Registration

For 2D rigid registration presented in Section 5 we compared $\mathcal{C}^{x}$, $\mathcal{C}^{u}_{\delta}$, $\mathcal{C}^{u}$, $\mathcal{C}^{x,u}_{\delta}$, and $\mathcal{C}^{x,u}$. Table I details the parameters used in each case.

| | $\mathcal{C}^{x}$ | $\mathcal{C}^{u}_{\delta}$ | $\mathcal{C}^{u}$ | $\mathcal{C}^{x,u}_{\delta}$ | $\mathcal{C}^{x,u}$ |
|---|---|---|---|---|---|
| $\kappa_{init}$ | ✗ | $\frac{5}{2^5}$ | $\frac{20}{2^5}$ | $\frac{5}{2^5}$ | $\frac{20}{2^5}$ |
| $\kappa_{step}$ | ✗ | 2 | 2 | 2 | 2 |
| $\kappa_{final}$ | ✗ | 5 | 20 | 5 | 20 |
| $h_{init}$ | $4^5 \times 0.007 \times c$ | ✗ | ✗ | $4^5 \times 0.007 \times c$ | $4^5 \times 0.007 \times c$ |
| $h_{step}$ | $\frac{1}{4}$ | ✗ | ✗ | $\frac{1}{4}$ | $\frac{1}{4}$ |
| $h_{final}$ | $0.007 \times c$ | ✗ | ✗ | $0.007 \times c$ | $0.007 \times c$ |

TABLE I
Parameters used for $\mathcal{C}^{u}$, $\mathcal{C}^{u}_{\delta}$, $\mathcal{C}^{x}$, $\mathcal{C}^{x,u}$ and $\mathcal{C}^{x,u}_{\delta}$ in our 2D rigid registration experiments. Here $c = \det(\frac{X^T X}{n_1})^{\frac{1}{2d}}$, where $X$ is the $n_1 \times d$ matrix of vertices in the model shape $S_1$.

### B. 2D Non-Rigid Registration

In Sections V and VII we also registered 2D shapes differing by a non-rigid deformation and the parameters used for $\mathcal{C}^{x}$, $\mathcal{C}^{x,u}$, $\mathcal{C}^{x}_{corr}$ and $\mathcal{C}^{x,u}_{corr}$ can be seen in Table II. In section V we also compared our results to the CPD and GLMD algorithms for non-rigid registration in 2D. The parameters used for the CPD method were the ones used by the authors in the code provided and can be seen in Table III. There were no parameters to set in the GLMD algorithm.

| | $\mathcal{C}^x$ | $\mathcal{C}^{x,u}$ | $\mathcal{C}^x_{corr}$ | $\mathcal{C}^{x,u}_{corr}$ |
|---|---|---|---|---|
| $\kappa_{init}$ | ✗ | $\frac{15}{2^4}$ | ✗ | $\frac{10}{1.5^4}$ |
| $\kappa_{step}$ | ✗ | 2 | ✗ | 1.5 |
| $\kappa_{final}$ | ✗ | 15 | ✗ | 10 |
| $h_{init}$ | $4^4 \times 0.007\times$ | $4^4 \times 0.007\times$ | $2^4 \times 0.007\times$ c | $2^4 \times 0.007\times$ c |
| $h_{step}$ | $\frac{1}{4}$ | $\frac{1}{4}$ | $\frac{1}{2}$ | $\frac{1}{2}$ |
| $h_{init}$ | $0.007\times$ c | $0.007\times$ c | $0.007\times$ c | $0.007\times$ c |

TABLE II
PARAMETERS USED FOR $\mathcal{C}^x$, $\mathcal{C}^{x,u}$ $\mathcal{C}^x_{corr}$ AND $\mathcal{C}^{x,u}_{corr}$ IN OUR EXPERIMENTS. HERE $c = \det(\frac{X^TX}{n_1})^{\frac{1}{2^d}}$, WHERE $X$ IS THE $n_1 \times d$ MATRIX OF VERTICES IN THE SHAPE $S_1$.

| CPD | |
|---|---|
| Outliers ($\omega$) | 0 |
| $\lambda$ | 2 |
| $\beta$ | 2 |
| Max Iter | 100 |
| Tolerance | $e^{-10}$ |

TABLE III
THE CPD PARAMETERS USED WHEN REGISTERING 2D SHAPES DIFFERING BY A NON-RIGID DEFORMATION, AS GIVEN IN THE CODE PROVIDED BY THE AUTHORS.

| | $\mathcal{C}^x$ | $\mathcal{C}^u_\delta$ | $\mathcal{C}^u$ | $\mathcal{C}^{x,u}_\delta$ | $\mathcal{C}^{x,u}$ |
|---|---|---|---|---|---|
| $\kappa_{init}$ | ✗ | $\frac{50}{2^{14}}$ | $\frac{25}{2^{14}}$ | $\frac{50}{2^7}$ | $\frac{25}{2^7}$ |
| $\kappa_{step}$ | ✗ | 2 | 2 | 2 | 2 |
| $\kappa_{final}$ | ✗ | 50 | 25 | 50 | 25 |
| $h_{init}$ | $2^7 \times 0.01\times$ c | ✗ | ✗ | $2^7 \times 0.01\times$ c | $2^7 \times 0.01\times$ c |
| $h_{step}$ | $\frac{1}{2}$ | ✗ | ✗ | $\frac{1}{2}$ | $\frac{1}{2}$ |
| $h_{final}$ | $0.01\times$ c | ✗ | ✗ | $0.01\times$ c | $0.01\times$ c |

TABLE IV
PARAMETERS USED FOR $\mathcal{C}^u$, $\mathcal{C}^u_\delta$ $\mathcal{C}^x$, $\mathcal{C}^{x,u}$ AND $\mathcal{C}^{x,u}_\delta$ IN OUR 3D RIGID REGISTRATION EXPERIMENTS WHEN THE SAME SAMPLING OF $S_1$ AND $S_2$ IS USED. HERE $c = \det(\frac{X^TX}{n_1})^{\frac{1}{2^d}}$, WHERE $X$ IS THE $n_1 \times d$ MATRIX OF VERTICES IN THE MODEL SHAPE $S_1$.

### *C. 3D Rotation Registration*

In Section VI, when testing several registration techniques on 3D data differing by a rigid transformation, we first explored the case in which the points sampled from $S_1$ and $S_2$ had exact correspondence pairs. The parameters used by our proposed cost functions can be seen in Table IV.

Next we registered shapes $S_1$ and $S_2$ that had no exact point correspondences. The parameters used in this case can be found in Table V. When registering shapes $S_1$ and $S_2$ when noise is added to $S_2$, we use the same parameters.

We also compared our results to the Go ICP and CPD methods. In both cases, the code and parameters provided by the authors was used and can be found in Table VI.

### *D. 3D Non-Rigid Registration*

In Section VI we tested $\mathcal{C}^{x,u}_{corr}$, $\mathcal{C}^x_{corr}$, CPD and GLMD when registering 3D shapes that differed by a non-rigid deformation. In our first experiment we used shapes that had exact point correspondences, and the parameters used for $\mathcal{C}^{x,u}_{corr}$ and $\mathcal{C}^x_{corr}$ are given in Table VII. We also tested these cost functions on 3D shapes with unknown correspondences that had to be estimated and the parameters used in this case can be seen in Table VIII. For both experiments, the CPD parameters used are those given in Table IX. Again, the GLMD setup used was that provided by the authors and no parameters needed to be set.

| | $\mathcal{C}^x$ | $\mathcal{C}^u_\delta$ | $\mathcal{C}^u$ | $\mathcal{C}^{x,u}_\delta$ | $\mathcal{C}^{x,u}$ |
|---|---|---|---|---|---|
| $\kappa_{init}$ | ✗ | $\frac{10}{2^7}$ | $\frac{25}{2^7}$ | $\frac{10}{2^7}$ | $\frac{25}{2^7}$ |
| $\kappa_{step}$ | ✗ | 2 | 2 | 2 | 2 |
| $\kappa_{final}$ | ✗ | 10 | 25 | 10 | 25 |
| $h_{init}$ | $2^7 \times 0.06\times$ c | ✗ | ✗ | $2^7 \times 0.06\times$ c | $2^7 \times 0.06\times$ c |
| $h_{step}$ | $\frac{1}{2}$ | ✗ | ✗ | $\frac{1}{2}$ | $\frac{1}{2}$ |
| $h_{final}$ | $0.06\times$ c | ✗ | ✗ | $0.06\times$ c | $0.06\times$ c |

TABLE V

PARAMETERS USED FOR $\mathcal{C}^u$, $\mathcal{C}^u_\delta$, $\mathcal{C}^x$, $\mathcal{C}^{x,u}$ AND $\mathcal{C}^{x,u}_\delta$ IN OUR 3D RIGID REGISTRATION EXPERIMENTS WITH DIFFERENT SAMPLING OF $S_1$ AND $S_2$, AND WITH ADDED NOISE TO THE POINTS $S_2$. HERE $c = \det(\frac{X^TX}{n_1})^{\frac{1}{2d}}$, WHERE $X$ IS THE $n_1 \times d$ MATRIX OF VERTICES IN THE SHAPE $S_1$.

| CPD | |
|---|---|
| Outliers ($\omega$) | 0.5 |
| Max Iter | 100 |
| Tolerance | $1e^{-8}$ |

| Go ICP | |
|---|---|
| MSE Threshold | 0.0001 |
| Trim Fraction | 0 |
| Nodes per dim | 300 |

TABLE VI

THE CPD AND GO ICP PARAMETERS USED WHEN REGISTERING 3D SHAPES DIFFERING BY A RIGID ROTATION, AS GIVEN IN THE CODE PROVIDED BY THE AUTHORS.

| | $\mathcal{C}^x_{corr}$ | $\mathcal{C}^{x,u}_{corr}$ |
|---|---|---|
| $\kappa_{init}$ | ✗ | $\frac{15}{2^5}$ |
| $\kappa_{step}$ | ✗ | 2 |
| $\kappa_{final}$ | ✗ | 15 |
| $h_{init}$ | $4^5 \times 0.0005\times$ c | $4^5 \times 0.0005\times$ c |
| $h_{step}$ | $\frac{1}{4}$ | $\frac{1}{4}$ |
| $h_{init}$ | $0.0005\times$ c | $0.0005\times$ c |

TABLE VII

PARAMETERS USED FOR $\mathcal{C}^x_{corr}$ AND $\mathcal{C}^{x,u}_{corr}$ IN OUR EXPERIMENTS WITH 3D SHAPES DIFFERING BY A NON-RIGID DEFORMATION WITH KNOWN CORRESPONDENCES. HERE $c = \det(\frac{X^TX}{n_1})^{\frac{1}{2d}}$, WHERE $X$ IS THE $n_1 \times d$ MATRIX OF VERTICES IN THE SHAPE $S_1$.

| | $\mathcal{C}^x_{corr}$ | $\mathcal{C}^{x,u}_{corr}$ |
|---|---|---|
| $\kappa_{init}$ | ✗ | $\frac{15}{2^5}$ |
| $\kappa_{step}$ | ✗ | 2 |
| $\kappa_{final}$ | ✗ | 15 |
| $h_{init}$ | $2^5 \times 0.001\times$ c | $2^5 \times 0.001\times$ c |
| $h_{step}$ | $\frac{1}{2}$ | $\frac{1}{2}$ |
| $h_{init}$ | $0.001\times$ c | $0.001\times$ c |

TABLE VIII

PARAMETERS USED FOR $\mathcal{C}^x_{corr}$ AND $\mathcal{C}^{x,u}_{corr}$ IN OUR EXPERIMENTS WITH 3D SHAPES DIFFERING BY A NON-RIGID DEFORMATION WITH UNKNOWN CORRESPONDENCES THAT NEEDED TO BE ESTIMATED. HERE $c = \det(\frac{X^TX}{n_1})^{\frac{1}{2d}}$, WHERE $X$ IS THE $n_1 \times d$ MATRIX OF VERTICES IN THE SHAPE $S_1$.

## V. ADDITIONAL SHAPE REGISTRATION RESULTS INCLUDING ALL COST FUNCTIONS

In Section III of the paper we propose cost functions $\mathcal{C}^u$, $\mathcal{C}^u_\delta$, $\mathcal{C}^{x,u}$ and $\mathcal{C}^{x,u}_\delta$ and when presenting the experimental results in Sections V and VI we omit the results of some of these cost functions for clarity as we found that both $\mathcal{C}^u_\delta$ and $\mathcal{C}^u$ performed similarly, as did $\mathcal{C}^{x,u}_\delta$ and $\mathcal{C}^{x,u}$. In this section, we provide similar results to those presented in Section V and VI of the paper for all four cost functions $\mathcal{C}^u$, $\mathcal{C}^u_\delta$, $\mathcal{C}^{x,u}$ and $\mathcal{C}^{x,u}_\delta$.

| CPD | |
|---|---|
| Outliers ($\omega$) | 0.1 |
| $\lambda$ | 3 |
| $\beta$ | 2 |
| Max Iter | 100 |
| Tolerance | $e^{-3}$ |

TABLE IX
THE CPD PARAMETERS USED WHEN REGISTERING 3D SHAPES DIFFERING BY A NON-RIGID DEFORMATION, AS GIVEN IN THE CODE PROVIDED BY THE AUTHORS.

### *A. 2D Rotation Registration*

In Figure 15 we present results similar to those in Figure 2 of the paper, in this case showing all cost functions $\mathcal{C}^u$, $\mathcal{C}^u_\delta$, $\mathcal{C}^{x,u}$ and $\mathcal{C}^{x,u}_\delta$. In Figure 15(a) we present the results when a rotation is estimated using the full curves, and we can see that $\mathcal{C}^u$ and $\mathcal{C}^u_\delta$ perform similarly, as do $\mathcal{C}^{x,u}$ and $\mathcal{C}^{x,u}_\delta$. In Figure 15(b) we present the results when a rotation is estimated using partial curves, with a percentage of points removed from the curve $S_1$. Again we can see that $\mathcal{C}^{x,u}$ and $\mathcal{C}^{x,u}_\delta$ perform similarly. While $\mathcal{C}^u_\delta$ seems to perform better than $\mathcal{C}^u$ in this case, both still perform better than $\mathcal{C}^x$ and worse than $\mathcal{C}^{x,u}$ and $\mathcal{C}^{x,u}_\delta$.

### *B. 3D Rotation Registration*

In Figure 16 we present results similar to those in Figure 4 of the paper, for all cost functions $\mathcal{C}^u$, $\mathcal{C}^u_\delta$, $\mathcal{C}^{x,u}$ and $\mathcal{C}^{x,u}_\delta$. From row 1 of Figure 16 we can see that CPD performs best when estimating a rotation when there are exact point correspondences between $S_1$ and $S_2$. Again both $\mathcal{C}^{x,u}$ and $\mathcal{C}^{x,u}_\delta$ perform similarly, as do $\mathcal{C}^u$ and $\mathcal{C}^u_\delta$, although $\mathcal{C}^u$ appears to get caught in alternate solutions at times, creating spikes in the average MSE results (Fig 16, row 1 and 2). When different samples are chosen from $S_1$ and $S_2$ (Fig 16, row 3) both $\mathcal{C}^{x,u}$ and $\mathcal{C}^{x,u}_\delta$ perform similarly, and both outperform $\mathcal{C}^x$. Both $\mathcal{C}^u$ and $\mathcal{C}^u_\delta$ also give similar results, performing the worst. The same results were found when registering shapes with added noise (Fig 16, row 4).

## REFERENCES


[1] J. Yang, H. Li, and Y. Jia, "Go-icp: Solving 3d registration efficiently and globally optimally," in *2013 IEEE International Conference on Computer Vision*, Dec 2013, pp. 1457–1464.

[2] A. Myronenko and X. Song, "Point set registration: Coherent point drift," *IEEE Transactions on Pattern Analysis and Machine Intelligence*, vol. 32, no. 12, pp. 2262–2275, Dec 2010.

[3] Y. Yang, S. H. Ong, and K. W. C. Foong, "A robust global and local mixture distance based non-rigid point set registration," *Pattern Recogn.*, vol. 48, no. 1, pp. 156–173, Jan. 2015. [Online]. Available: http://dx.doi.org/10.1016/j.patcog.2014.06.017

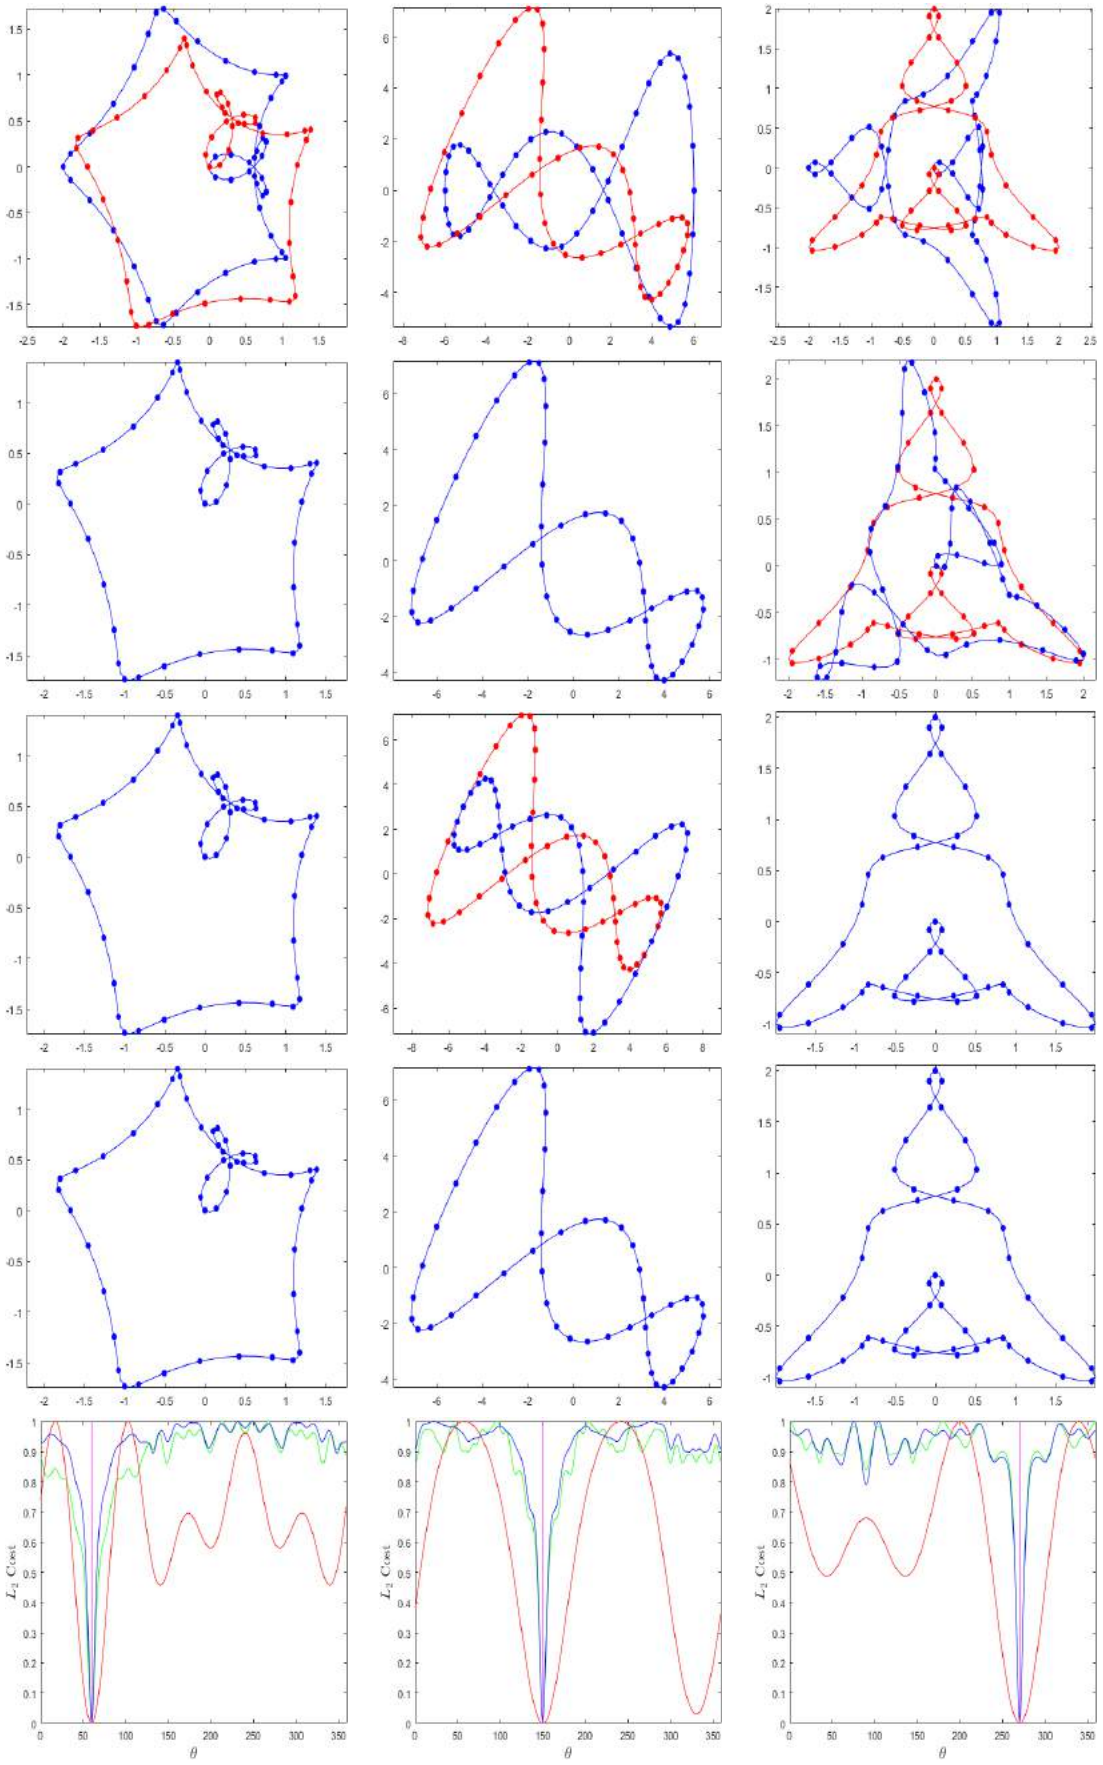

Fig. 2. Sample registration results for rotation estimation with 2D data. Row 1: Model Curve (blue) and Target Curve (red). Row 2 - 4: Registration result using $\mathcal{C}^x$, $\mathcal{C}^u$ and $\mathcal{C}^{x,u}$ respectively. Row 5 shows the value of each of the cost functions when $\theta$ ranges from 1°to 360°. In these graphs red represents $\mathcal{C}^u$, green represents $\mathcal{C}^x$ and blue represents $\mathcal{C}^{x,u}$. The pink line indicates the value of $\theta_{GT}$.

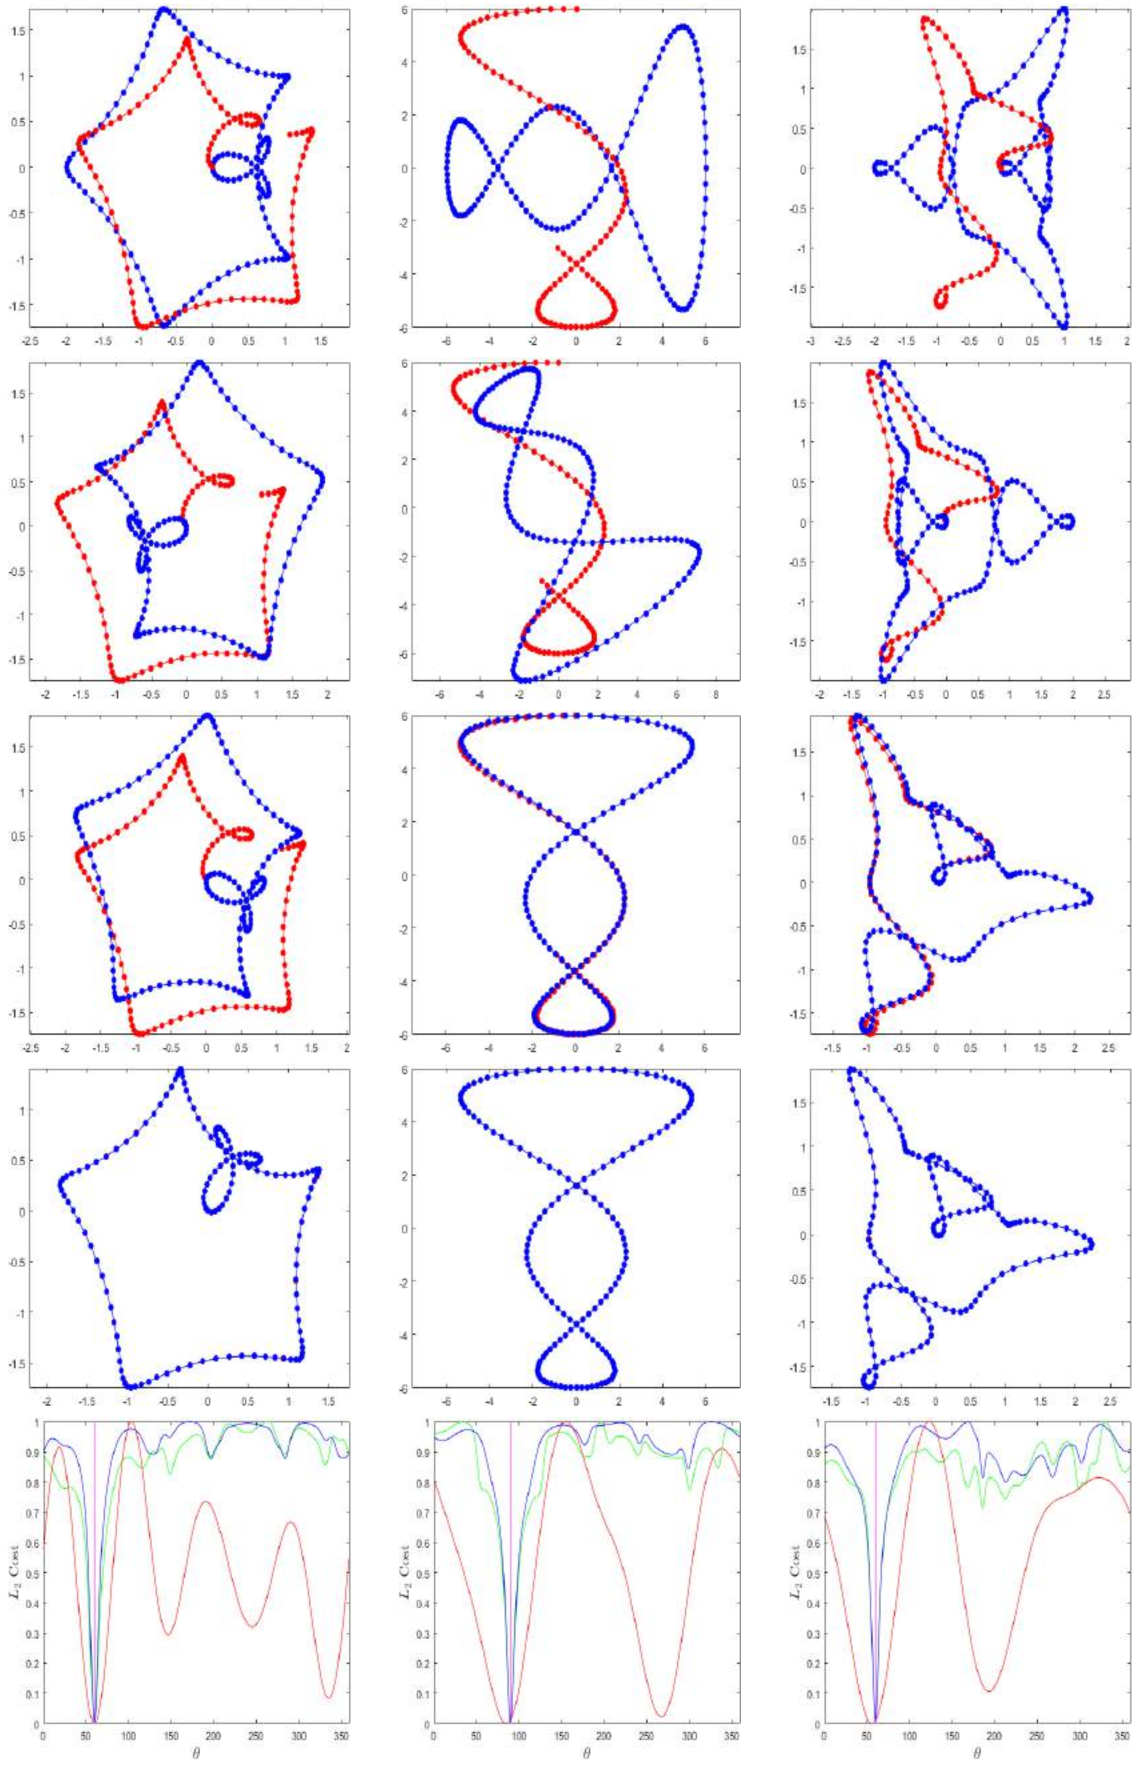


Fig. 3. Sample registration results for rotation estimation with missing data. Row 1: Model Curve (blue) and Target Curve (red). Row 2 - 4: Registration result using $\mathcal{C}^x$, $\mathcal{C}^u$ and $\mathcal{C}^{x,u}$ respectively. Row 5 shows the value of each of the cost functions when $\theta$ ranges from $1^\circ$to $360^\circ$. In these graphs red represents $\mathcal{C}^u$, green represents $\mathcal{C}^x$ and blue represents $\mathcal{C}^{x,u}$. The pink line indicates the value of $\theta_{GT}$.

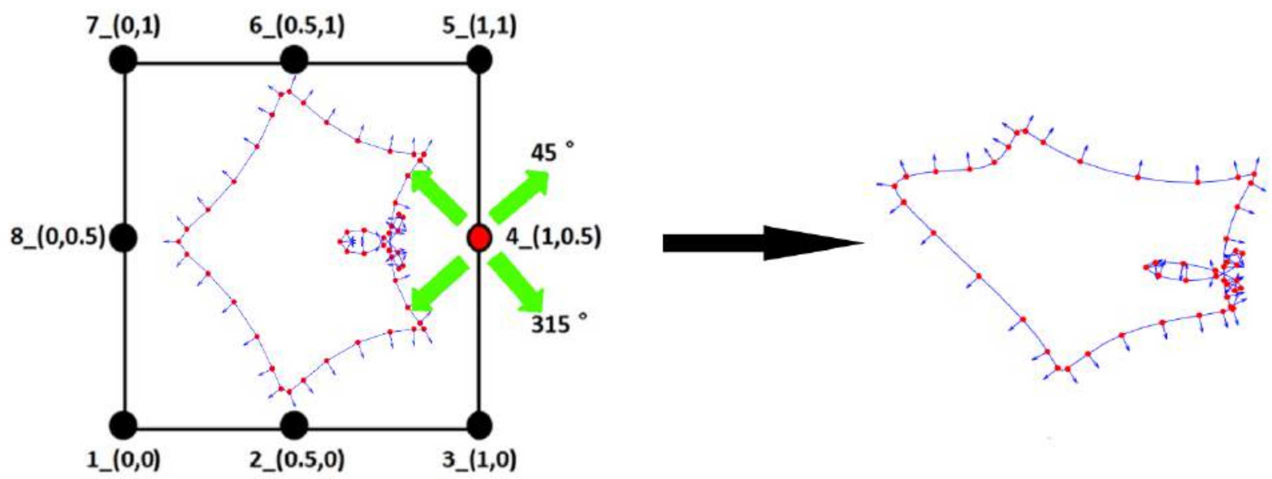


Fig. 4. On the left we show the 8 control points chosen on the boundary of the shape $S_2$ which can move in any four directions (shown in green). The deformed control points are used to estimate a transformation which deforms $S_2$, creating $S_1$ (right).

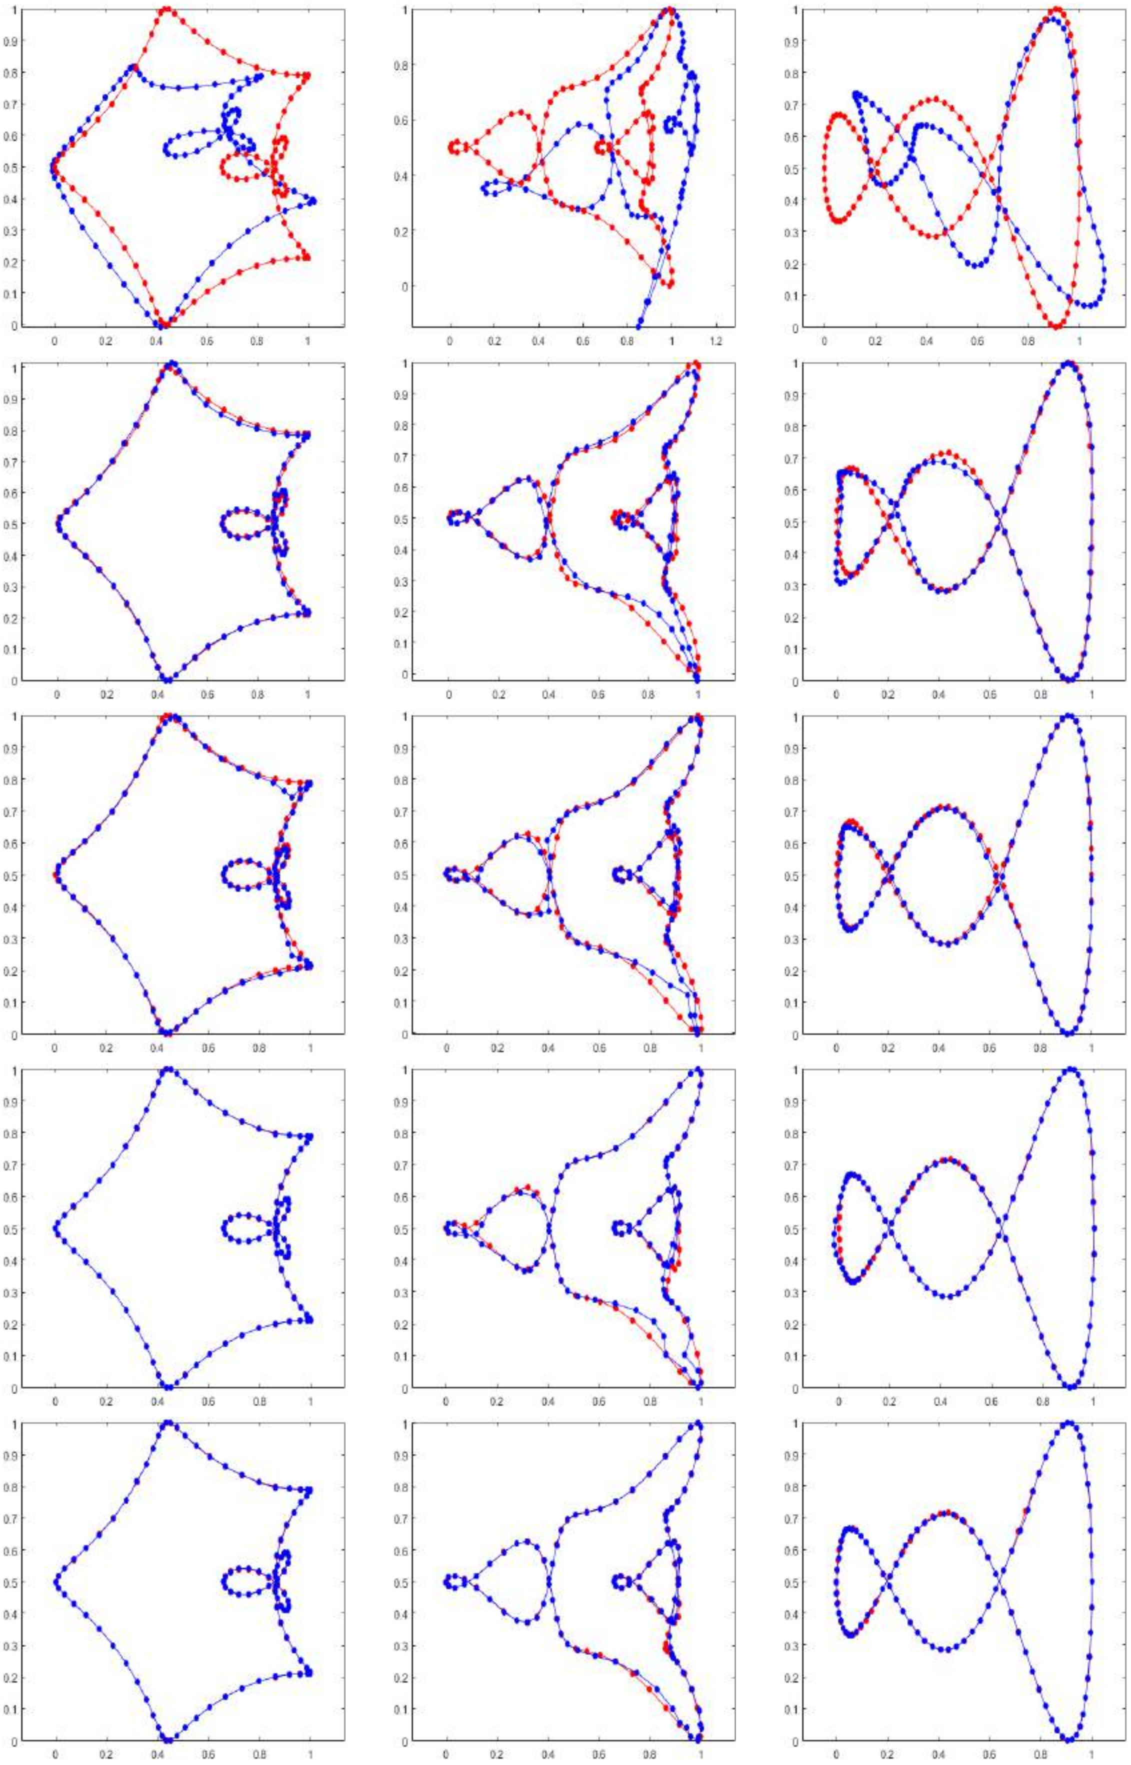

Fig. 5. Sample registration results for deformation estimation. Row 1: Model Curve (blue) and Target Curve (red). Row 2 - 5: Registration result using CPD, GLMD, $\mathcal{C}^{x}$ and $\mathcal{C}^{x,u}$ respectively. Column 1: Deformation degree = 5; Column 2: Deformation degree = 6; Column 3: Deformation degree = 8;

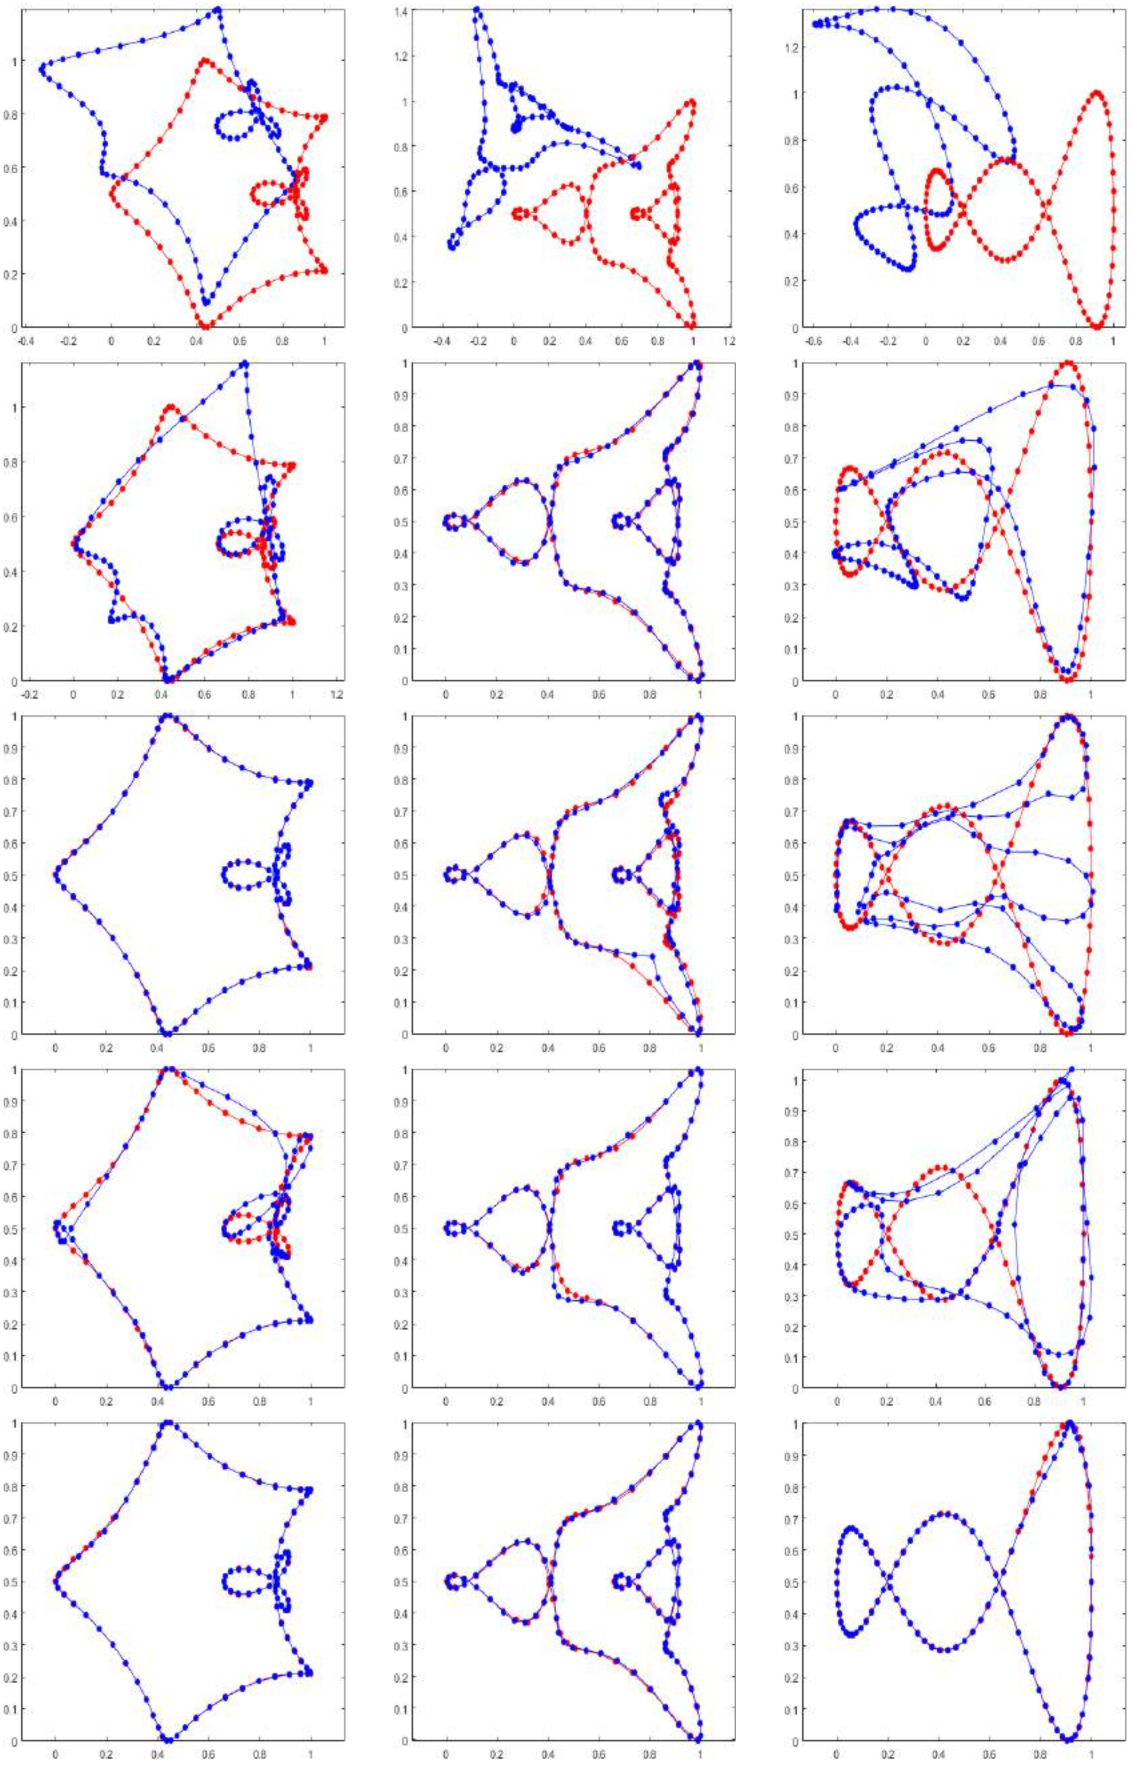

Fig. 6. Sample registration results for rotation and deformation estimation. Row 1: Model Curve (blue) and Target Curve (red). Row 2 - 5: Registration result using CPD, GLMD, $\mathcal{C}^{x}$ and $\mathcal{C}^{x,u}$ respectively. Column 1: Rotation = 30 $^\circ$; Column 2: Rotation = 45 $^\circ$; Column 3: Rotation = 60 $^\circ$.

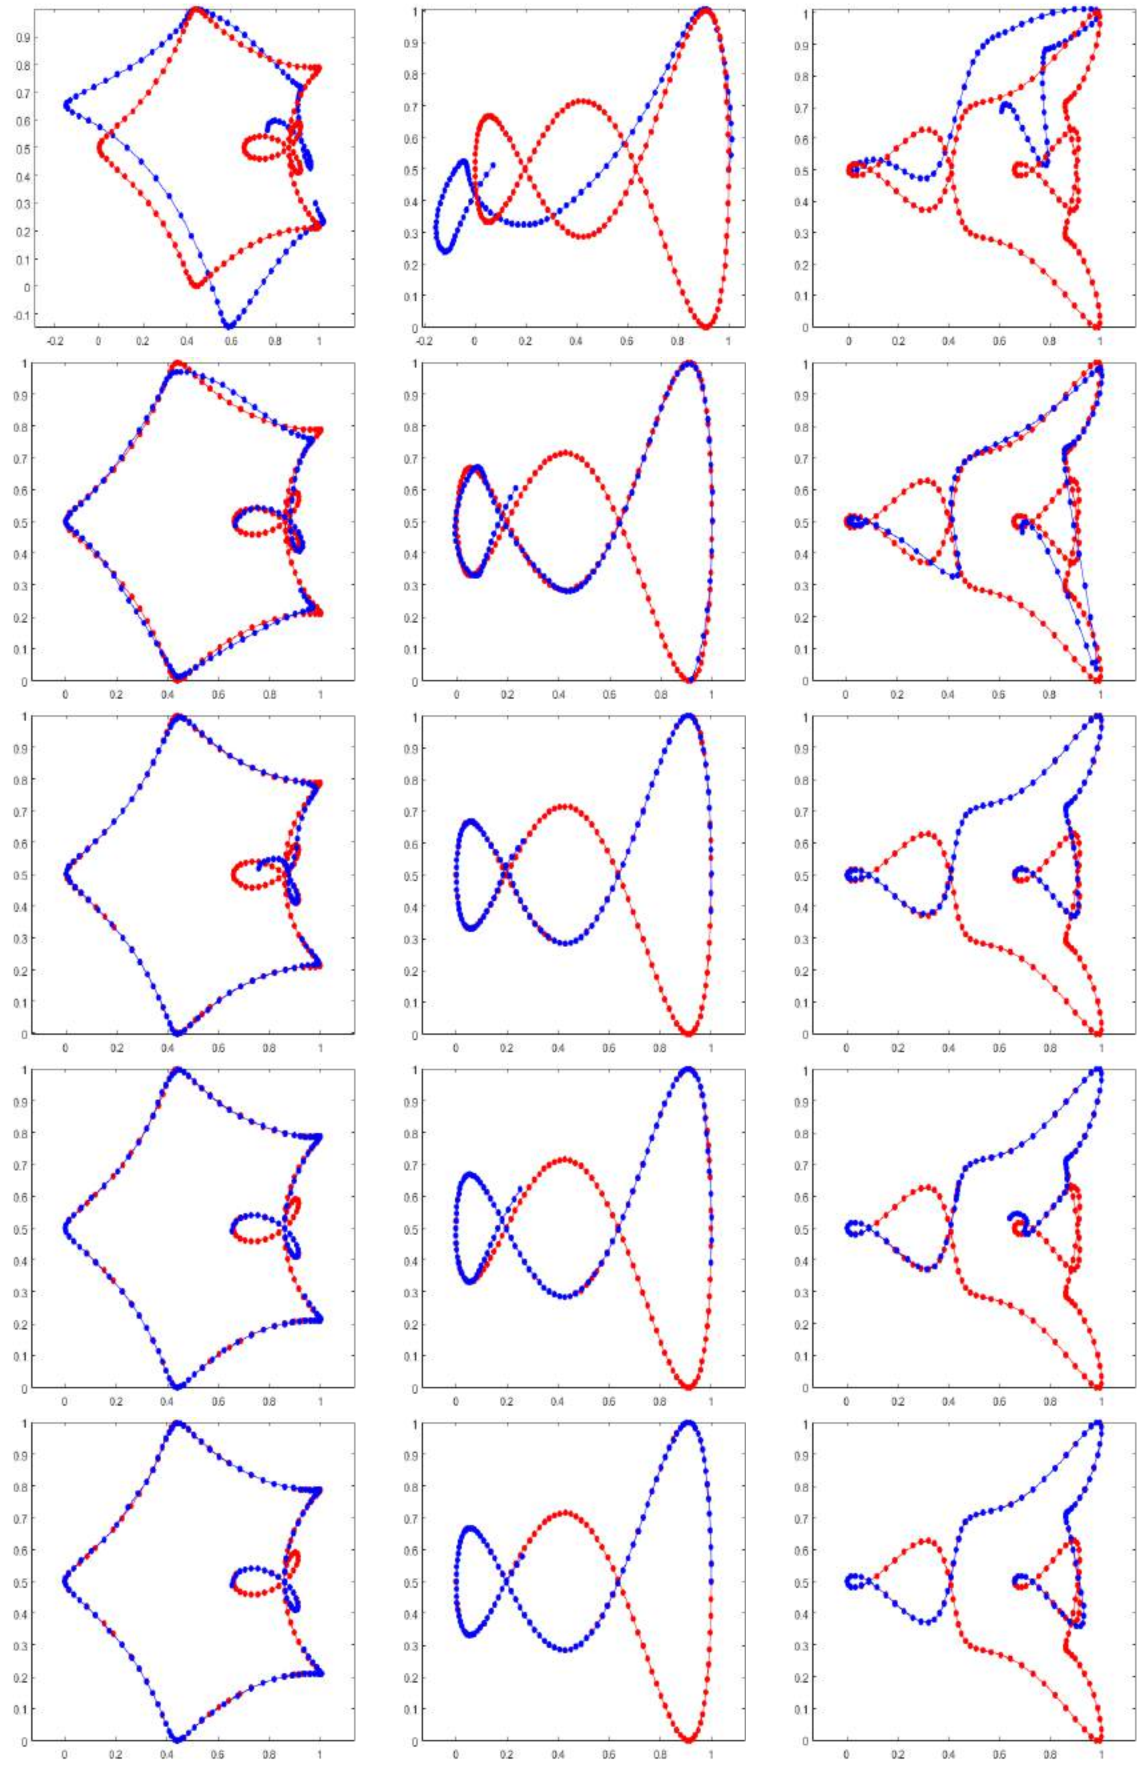

Fig. 7. Sample registration results for deformation estimation with missing data. Row 1: Model Curve (blue) and Target Curve (red). Row 2 - 5: Registration result using CPD, GLMD, $\mathcal{C}^{x}$ and $\mathcal{C}^{x,u}$ respectively. Column 1: Missing pts = 30; Column 2:Missing pts = 50; Column 3:Missing pts = 70.

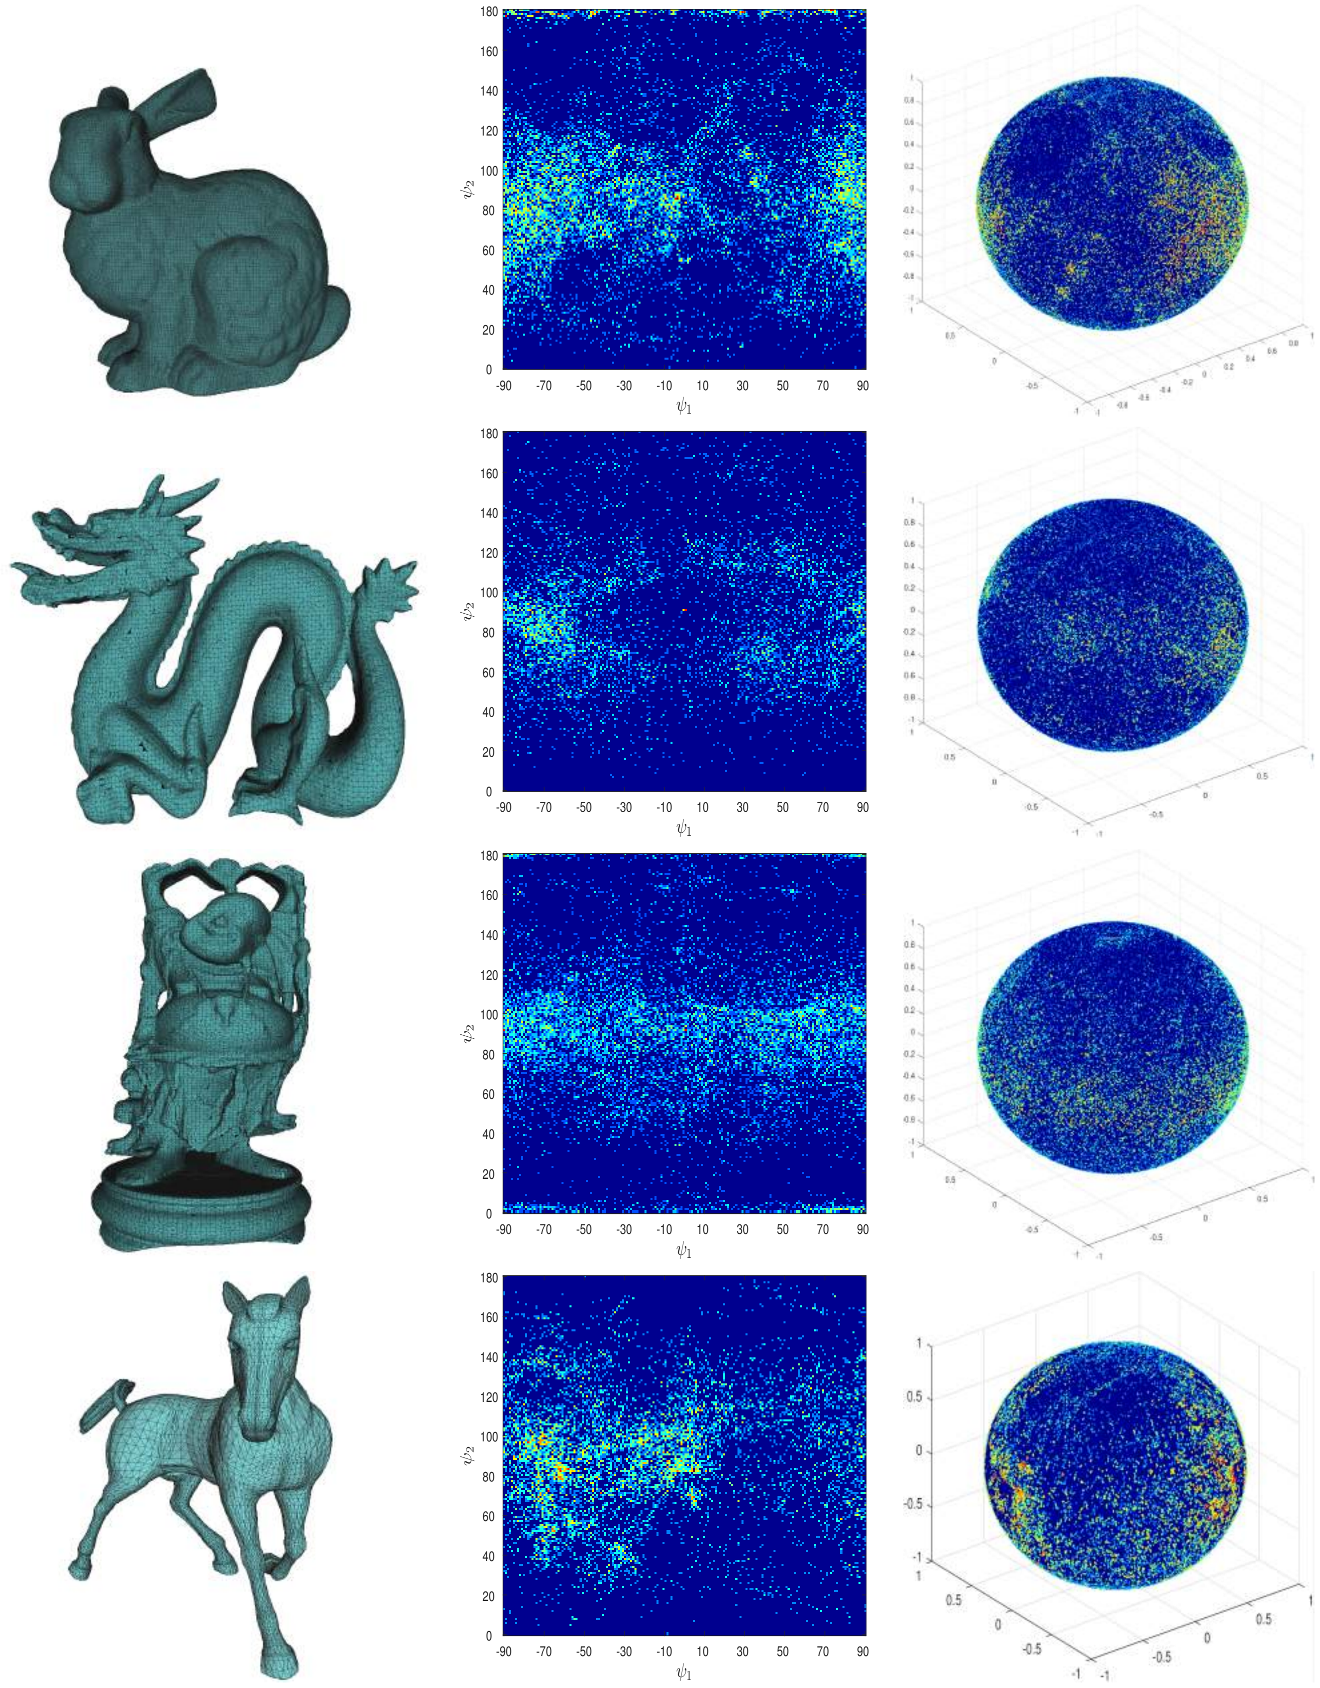


(a) (b) (c)

Fig. 8. Column (a) shows the Bunny, Dragon Buddha and Horse meshes. Column (b) shows the distribution of normal vectors for each mesh in 2D. The normals can be parametrised as $u(\psi_1, \psi_2) = (\cos(\psi_1)\cos(\psi_2),\, \sin(\psi_1)\cos(\psi_2),\, \sin(\psi_2))$. Column (c) shows the distribution of normal vectors $u^{(i)}$ on the sphere.

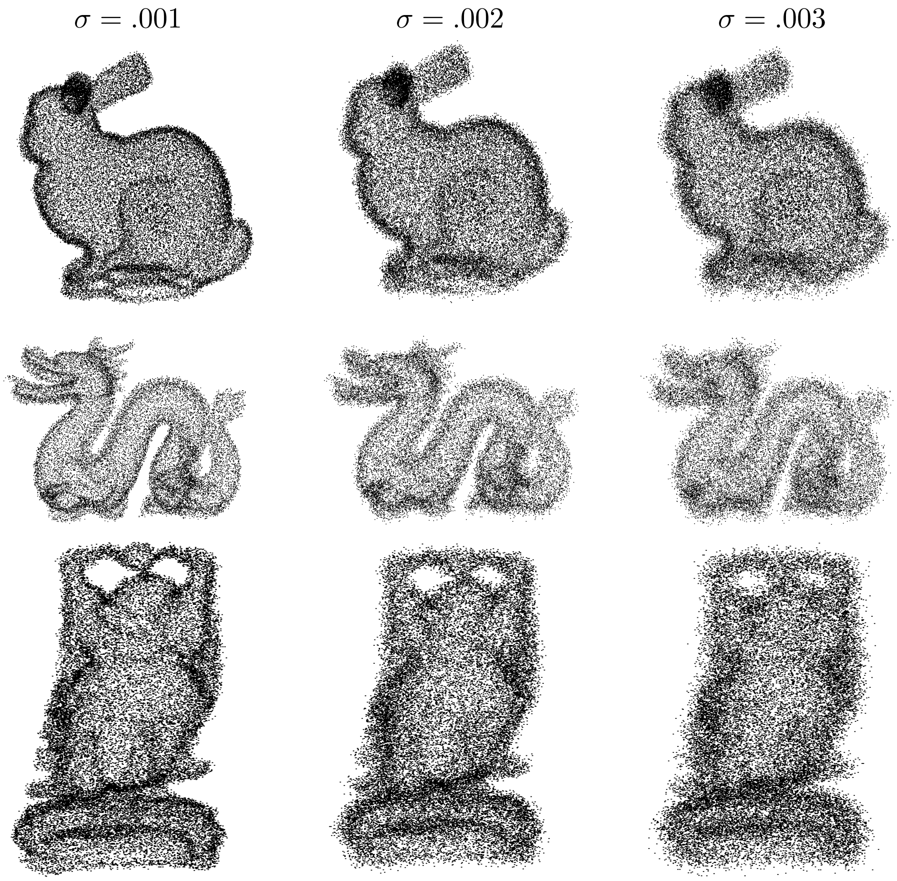


Fig. 9. Here we show the noisy points $\{x_2^{(i)}\}$ when $S_2$ corresponds to the Bunny, Dragon and Buddha shapes. Gaussian noise of mean 0 and standard deviation $\sigma$ is added to each point $x^{(i)}$. Column 1: $\sigma = 0.001$, Column 2: $\sigma = 0.002$, Column 3: $\sigma = 0.003$.

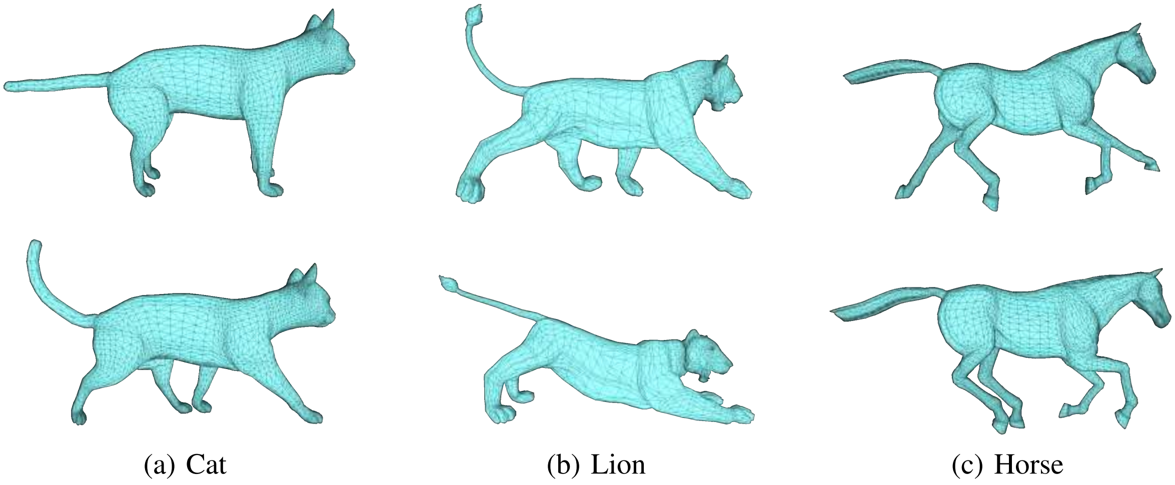


Fig. 10. The meshes used to generate the shapes $S_1$ and $S_2$ in our non-rigid registration experiment on 3D data. Meshes representing the same animal (eg. cat, lion, horse) have the same number of vertices and exact vertex correpondences. The cat, lion and horse meshes have 7202, 5000 and 8431 vertices respectively.

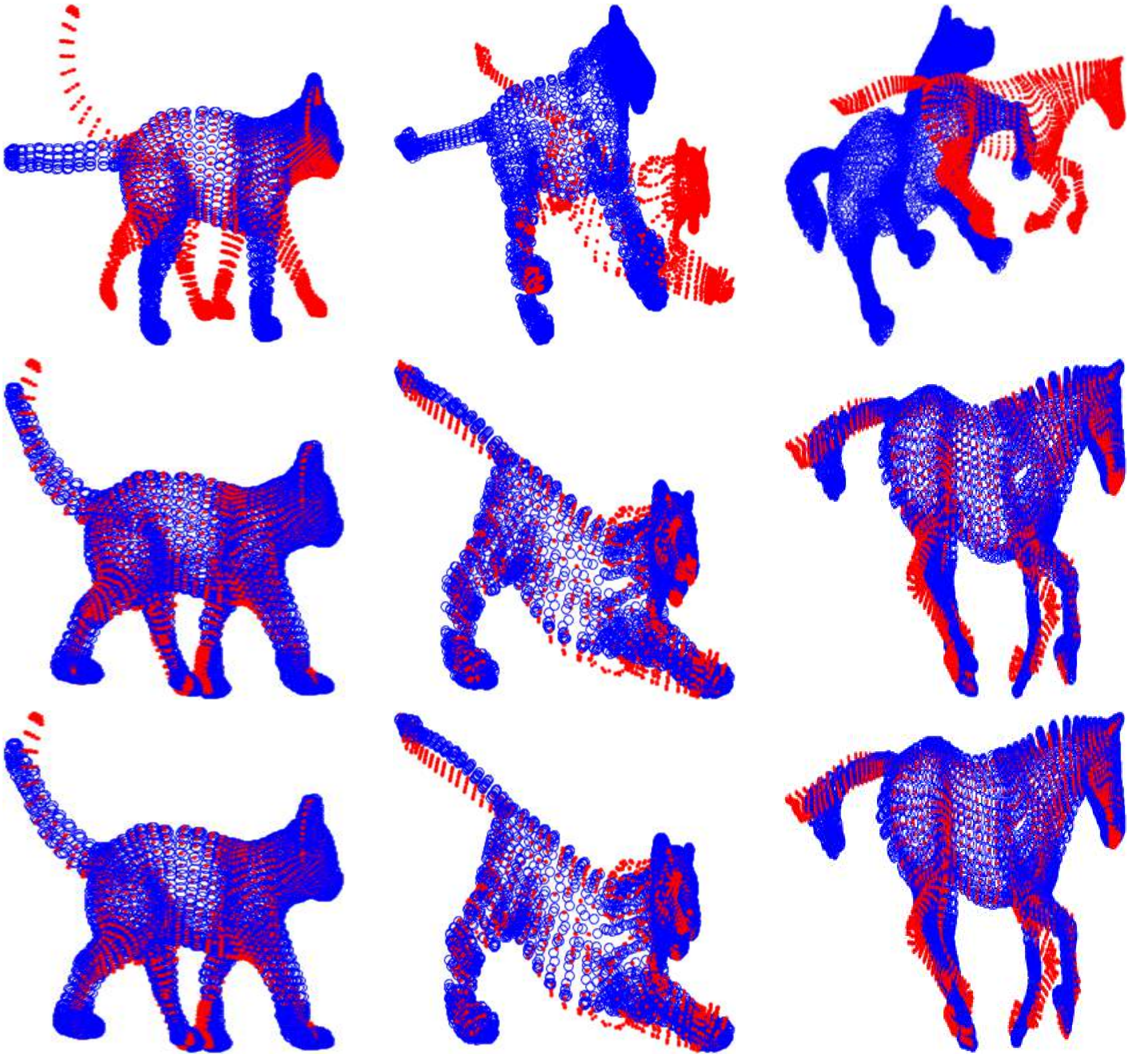

(a)Rotation $0^{\circ}$ (b)Rotation $20^{\circ}$ (c) Rotation $40^{\circ}$

Fig. 11. Some of the registration results for $\mathcal{C}_{Corr}^{x}$ and $\mathcal{C}_{Corr}^{x,u}$ for shapes with exact point correspondences. Row 1: The model shape $S_1$ (blue) and target shape $S_2$ (red); Row 2: Target shape (red) and $\mathcal{C}_{Corr}^{x}$ registration results (blue); Row 3: Target shape (red) and $\mathcal{C}_{Corr}^{x,u}$ registration results (blue).

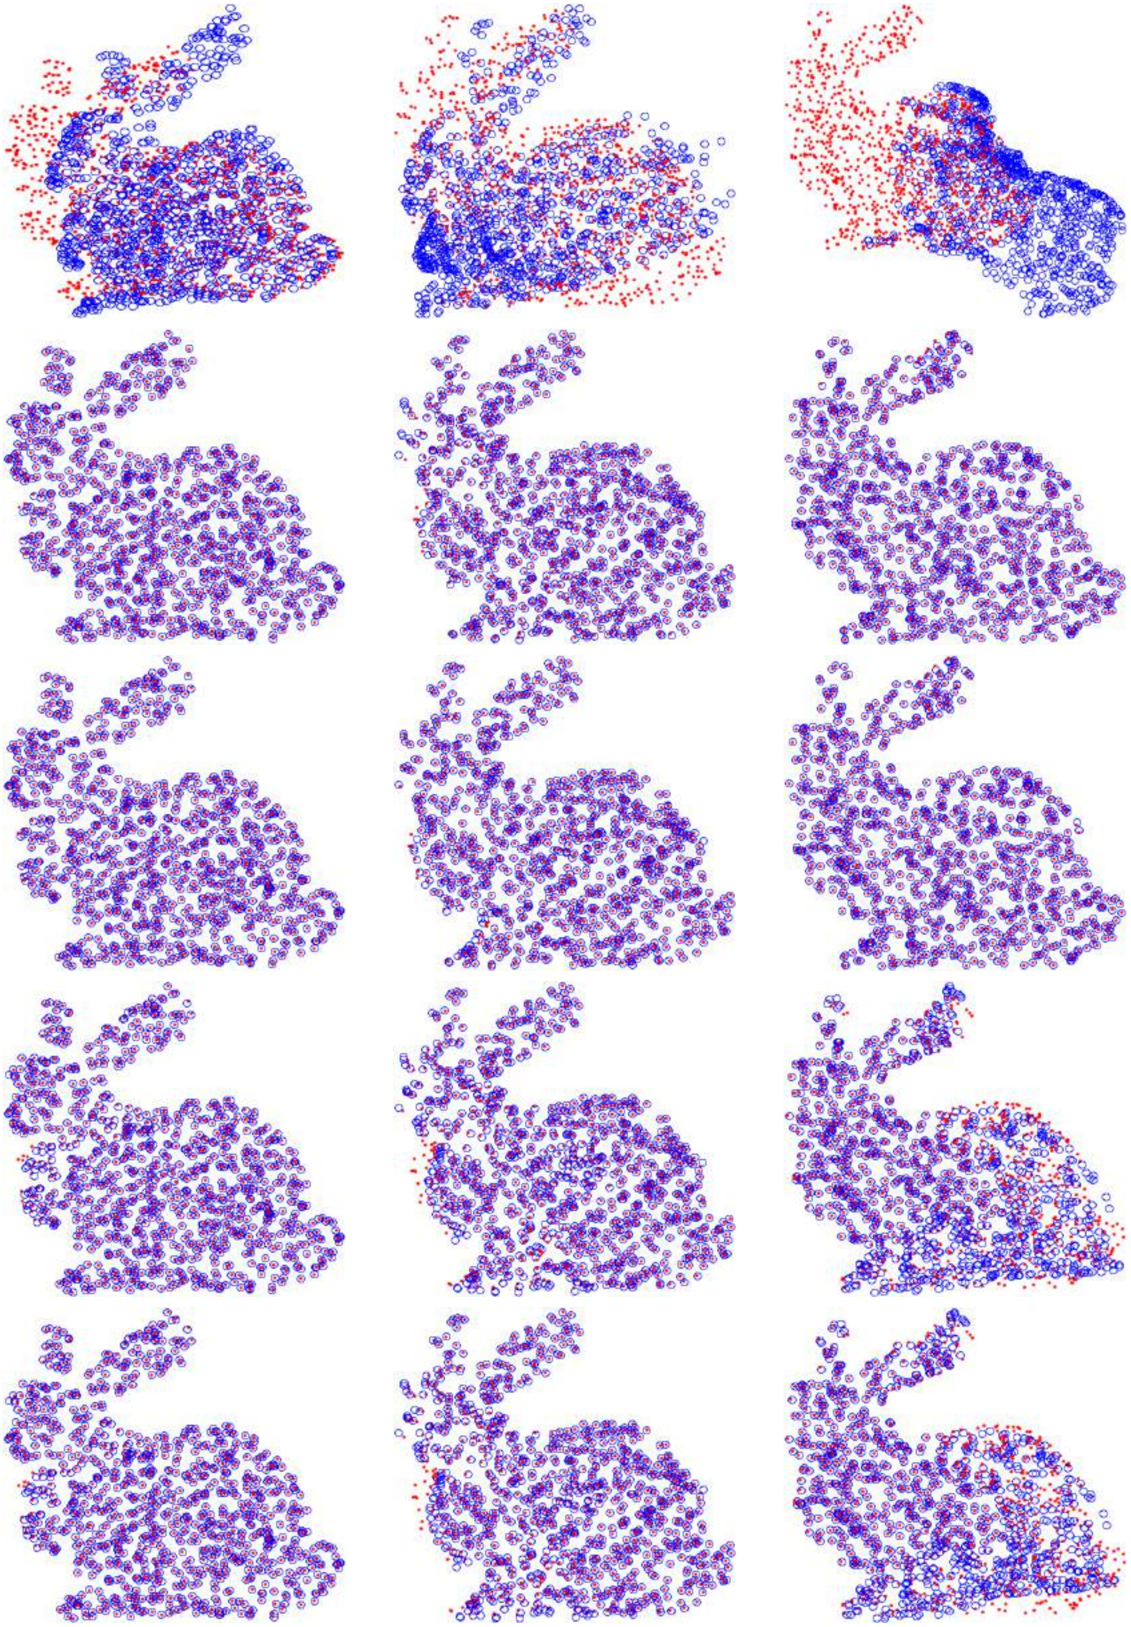

Rotation = $0°$ | Rotation = $0°$ | Rotation = $45°$

Deformation Degree = 2 | Deformation Degree = 4 | Deformation Degree = 3

Fig. 12. The results of several registration methods applied to two 3D shapes differing by a non-rigid deformation and a rotation. Row 1 shows the model shape $S_1$ (blue) and target shape $S_2$ (red). Rows (2 - 5) show the transformed model after registration (blue) computed using CPD (Row 2), GLMD (Row 3), $\mathcal{C}^{x}_{corr}$ (Row 4) and $\mathcal{C}^{x,u}_{corr}$ (Row 5).

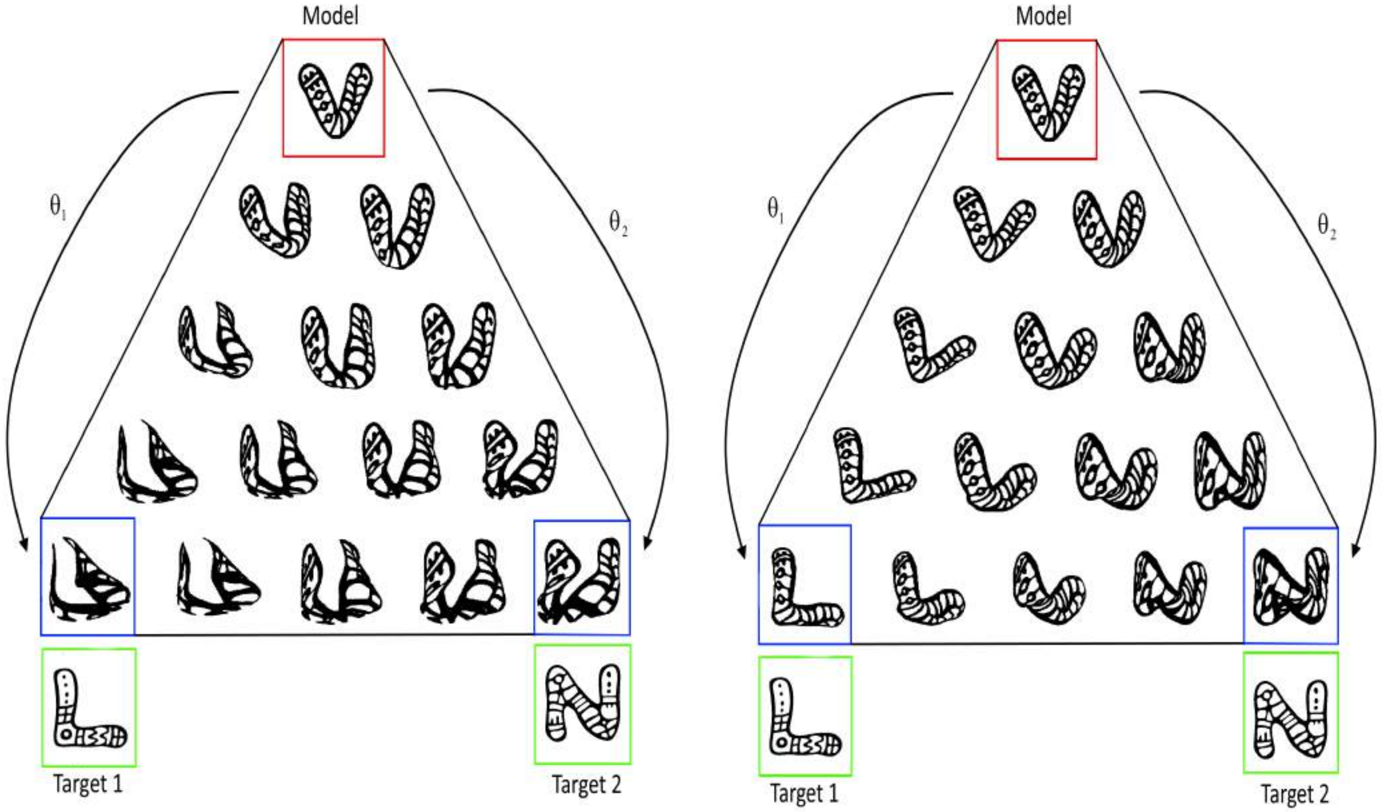


(a) Using $\mathcal{C}^x$

(b) Using $\mathcal{C}^{x,u}$

Fig. 13. Curve registration and interpolation results generated using (a) $\mathcal{C}^x$ and (b) $\mathcal{C}^{x,u}$. In both cases, $\mathcal{C}^x$ and $\mathcal{C}^{x,u}$ are used to register the model letter 'V' (red) to target letters 'L' and 'N' (green). The registration results after transformation using the estimated parameters $\theta_1$ and $\theta_2$ are outlined in blue, showing that $\mathcal{C}^{x,u}$ performs better than $\mathcal{C}^x$ when registering 'V' to 'L' and 'N'. In both cases, new shapes can be created by interpolating between the model shape 'V' and its transformations into 'L' and 'N'. These are shown in the pyramids.

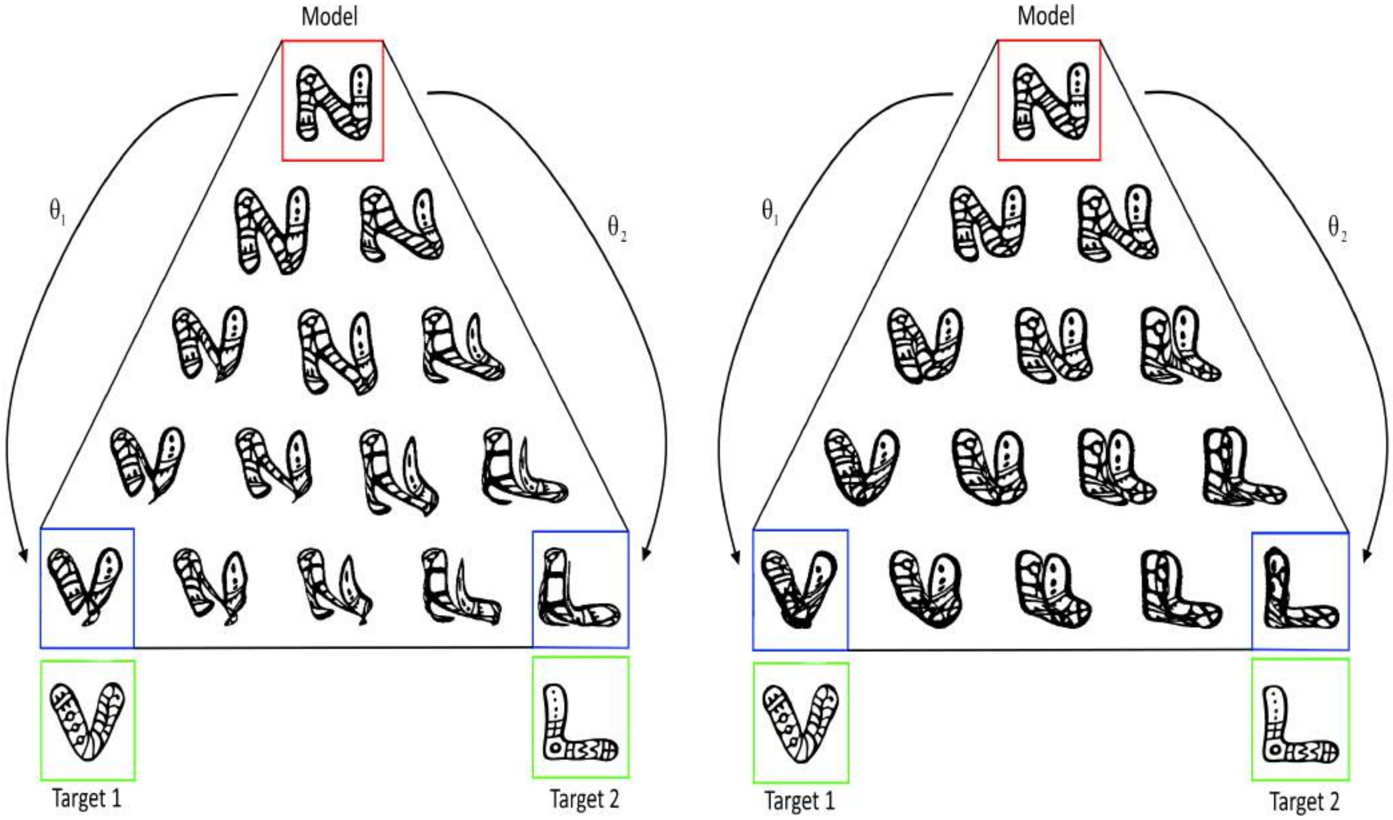


(a) Using $\mathcal{C}^x$ (b) Using $\mathcal{C}^{x,u}$

Fig. 14. Curve registration and interpolation results generated using (a) $\mathcal{C}^x$ and (b) $\mathcal{C}^{x,u}$. In both cases, $\mathcal{C}^x$ and $\mathcal{C}^{x,u}$ are used to register the model letter 'N' (red) to target letters 'V' and 'L' (green). The registration results after transformation using the estimated parameters $\theta_1$ and $\theta_2$ are outlined in blue, showing that $\mathcal{C}^{x,u}$ performs better than $\mathcal{C}^x$ when registering 'N' to 'V' and 'L'. In both cases, new shapes can be created by interpolating between the model shape 'N' and its transformations into 'V' and 'L'. These are shown in the pyramids.

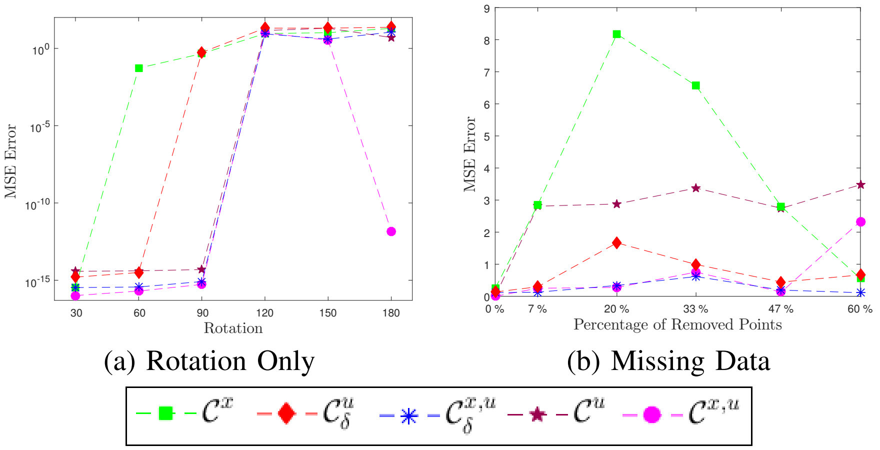


(a) Rotation Only (b) Missing Data

Fig. 15. MSE results for each of our experiments on 2D data differing by a rotation. In (a) the MSE value given at each rotation is the average over 10 curve registration results, as is the MSE value given at each percentage of removed points in (b).

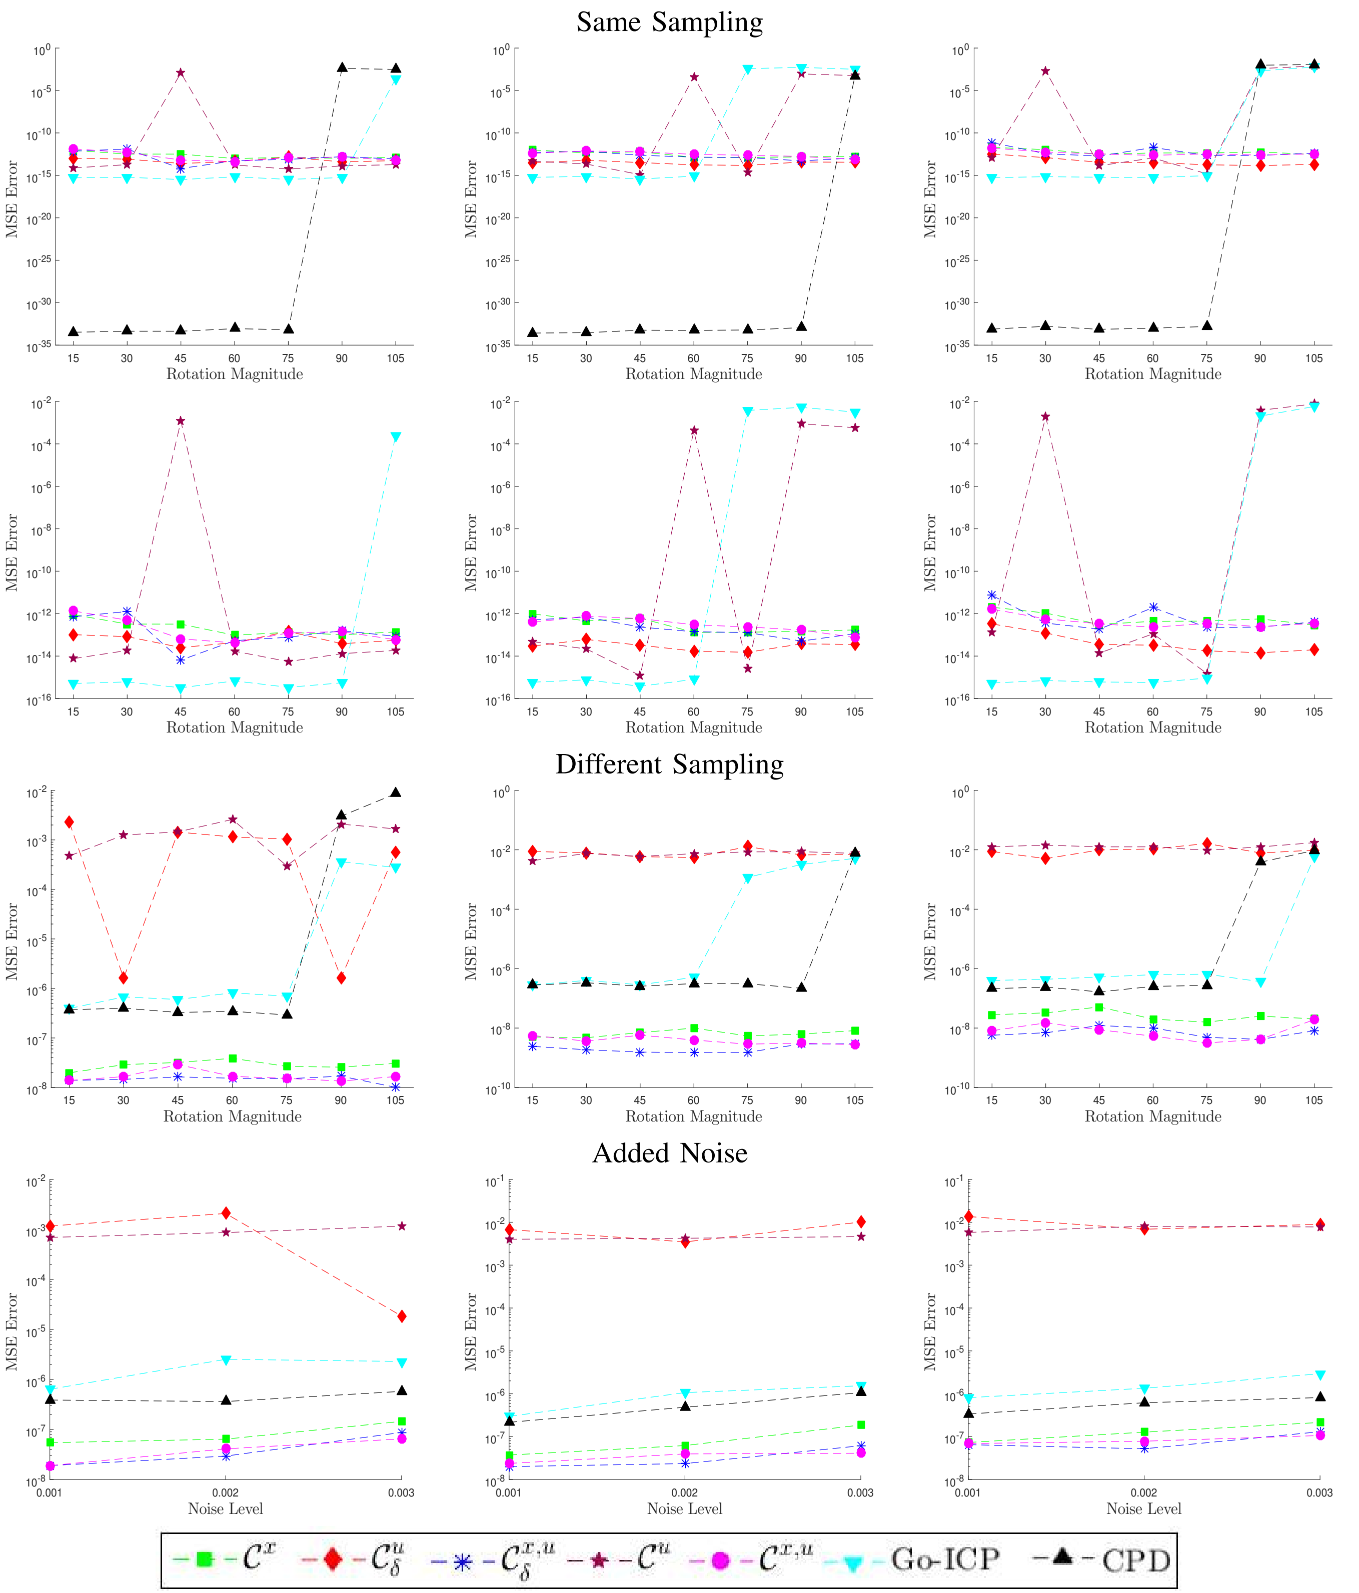


(a) Bunny (b) Dragon (c) Buddha

Fig. 16. Error results obtained when registering shapes $S_1$ and $S_2$ with the same sampling (row 1), omitting CPD for clarity (row 2), registering shapes with different sampling (row 3) and with added noise (row 4). Columns 1-3 give the error results for the Bunny, Dragon and Buddha meshes respectively.
